# Supplementary material for: Naive Feature Selection: a Nearly Tight Convex Relaxation for Sparse Naive Bayes
Source: arXiv:1905.09884 source file (2025-03-12)
Supplement: Supplementary file 1 [file appendixD.tex]

\section{Robustness} \label{subsec:rob} 
In this section we consider a variant of the original naive Bayes models where the input data (matrix $X$) is imperfectly known, and subject to adversarial noise.  We adopt the robust maximum likelihood (maximin) principle developed in~\citet{ben2009robust,lanckriet2002robust,bertsimas2019robust}. 

\subsection{Robust maximum likelihood}
Consider a generic maximum likelihood problem
\[
\max_\theta \: \mathcal{L}(\theta; X),
\]
with $X \in \reals^{n \times m}$ the data matrix, $\mathcal{L}$ the loss function and $\theta \in \reals^m$ containing the parameters of the model.

We now assume that $X$ is subject to additive noise. Modeling the noisy matrix as $X+U$, where matrix $U$ is only known to belong to a given ``uncertainty set'' ${\cal U} \subseteq \reals^{n \times m}$, the robust version of the above problem is defined as
\begin{equation}\label{eq:rob-maximin}
    \max_\theta \: \min_{U \in {\cal U}} \: \mathcal{L}(\theta; X+U),
\end{equation}
where $\mathcal{L}$ is the loss function and $\theta \in \reals^m$ contains the parameters of the model.  Note that the approach generalizes well-known models, for example with the loss function $\mathcal{L}(\theta; X) = -\|X\theta - y\|_2$, with $y \in \reals^n$ a given response vector, and the uncertainty set ${\cal U}$ chosen to be the set of matrices with largest singular value norm less than a given positive number $\rho$, the resulting robust counterpart is the so-called ``square-root'' version of ridge regression:
\[
\max_\theta \: -\|X\theta-y\|_2 - \rho \|\theta\|_2.
\]
This illustrates the connections between robust counterparts and penalization, with a penalty that depends specifically on the uncertainty set, as further elaborated in \citet{ben2009robust}.  We will observe a similar connection in the context of naive Bayes.

We now consider such robust formulations of \eqref{eq:bnb_train} and \eqref{eq:mnb_train}. First, we define noise models that make sense from a practical point of view.

\subsection{Adversarial noise models}
We assume that the uncertainty affects each data point independently. This leads to uncertainty sets of the form 
\[
{\cal U}(X) = \left\{ [u_1, \ldots,u_n] \in \reals^{n \times m} ~:~ u_i \in {\cal V}(x_i) , \;\; i \in [n] \right\},
\]
where a set ${\cal V}(x) \subseteq \reals^m$ models the uncertainty on a generic data point $x \in \reals^n$. We focus on the following uncertainty sets, depending on the nature of the data point, either binary-, integer-, or real-valued. 

In the Bernoulli model, the input is binary, so it makes sense to consider flips as a primary source of uncertainty. For a given binary vector $x \in \{0,1\}^n$ and integer $p \in [m]$,
\begin{align}\label{eq:unc-bnb}
    {\cal V}_\text{flip}(x) &= \{ \delta ~:~ \delta + x \in \{0,1\}^m, \;\; \|\delta\|_1 \leq p\} . \tag{$p$-flips}  
\end{align}
Thus, ${\cal V}_\text{flip}(x)$ represents the set of vectors that can be obtained by flipping at most $p\leq m$ components in a binary vector $x$. 

For the multinomial model, we often deal with count vectors $x \in \mathbb{N}^n$. The set
\begin{align}\label{eq:unc-mnb}
   {\cal V}_\text{typo}(x) &= \{ \delta ~:~ \delta + x \in \mathbb{N}^m, \|\delta\|_1 \leq t\} \tag{$t$-typos}
\end{align}
models the fact that count vectors can be altered by adding or substracting at most $t$ counts to $x$. This can represent the presence of typos in text data.

Finally, for a real-valued vector $x \in \reals^n$:
\begin{align}\label{eq:unc-lmbda}
    {\cal V}_\text{shift}(x) &= \{ \delta ~:~ \delta + x \in \mathbb{N}^m, \delta \in [-\gamma, \gamma]^m\cap \mathbb{Z}^m \} , \tag{$\gamma$-shift}
\end{align}
with $\gamma>0$ given. Here, ${\cal V}_\text{shift}(x)$ represents an interval uncertainty affecting each feature independently.

\subsection{Robust counterparts}
Applying the modified formulation~\eqref{eq:rob-maximin} in lieu of the classical naive Bayes ones \eqref{eq:bnb_train} and \eqref{eq:mnb_train} leads to, respectively:
\begin{align} \label{eq:r-bnb-flip}
&\max_{\tp, \tm \in [0,1]^m} \:
\min_{U \in {\cal U}_\text{flip}(X)} \: \mathcal{L}_{\text{bnb}}(\tp,\tm; X+U) , \tag{R-BNB-flip} 
\end{align}
and 
\begin{align}\label{eq:r-mnb}
&\max_{\tp, \tm \in [0,1]^m} \:
\min_{U \in {\cal U}(X)} \:
\mathcal{L}_{\text{mnb}}(\tp,\tm; X+U)  ~:~ \ones^\top \tp = \ones^\top\tm = 1,\tag{R-MNB}
\end{align}
where ${\cal U}(X)$ is one of the uncertainty sets introduced above, with the exception of the first \eqref{eq:unc-bnb}.

The inner minimization can be solved exactly for all the proposed uncertainty sets. Below we derive the subsequent robust, convex optimization problems corresponding to each of the uncertainty sets.

% The following result illustrates this for one of the uncertainty models. 

% \begin{theorem}\label{thm:rob}
% In the ``typo'' uncertainty set given by \eqref{eq:unc-mnb}, the robust variant of naive Bayes \eqref{eq:r-mnb} reduces to a convex optimization problem:
% \begin{align*}
% \displaystyle\max_{\tp, \tm \in [0,1]^m} & \fpt \log \tp +  \fmt \log \tm -t \Big(\log (\dsp\max_{1 \le i \le m} \: \tp_i) + \log (\dsp\max_{1 \le i \le m} \: \tm_i)\Big) \\
% &\text{s.t} ~~ \ones^\top \tp = \ones^\top \tm = 1
% \end{align*}
% \end{theorem}

% \section*{Proof of Theorem \eqref{thm:rob}}

\paragraph{Bernoulli model with flip uncertainty.}
Under $p$-flip uncertainty, \eqref{eq:r-bnb-flip} becomes
\begin{align*}
    \max_{\tpm\in[0,1]^m} \: \min_{\delta_\pm \in R_\pm} &(\fp+\delta_+)^\top \log \tp + (\ones - (\fp + \delta_-))^\top \log (\ones - \tp) \\
    &+ (\fm+\delta_-)^\top \log \tm + (\ones - (\fm+\delta_-))^\top \log (\ones - \tm) ,
\end{align*}
where for given $f \in \{0,1\}^m$
\[
R(f) := \left\{\delta ~:~ \delta + f \in \{0,1\}^m, \;\; \|\delta\|_1 \leq p \right\}.
\]
First analyze the following sub-problem, for given $\theta \in (0,1)^m$ and $f \in \{0,1\}^m$:
\begin{align}\label{eq:r-decomp}
    &\min_{\delta \in R(f)} \: (f+\delta)^\top \log \theta + (\ones - (f + \delta))^\top \log (\ones - \theta)  \\&= f^\top \log \theta +
    (\ones-f)^\top \log(\ones - \theta) + \min_{\delta \in R(f)} \: \delta^\top q(\theta) , \nonumber
\end{align}
where $q(\theta):= \log \theta - \log (\ones -\theta)$.

Since $f \in \{0,1\}^m$, the constraint $\delta + f \in \{0,1\}^m$ implies that $\delta \in \{-1,0,1\}^m$. For given $i \in [m]$, if $f_i = 0$ then $\delta_i \in \{0,1\}$ and if $f_i = 1$ then $\delta_i \in \{-1,0\}$. Then for $q \in \reals^m$ given, define
\begin{align}
    h(q;f) &:= \min_{\delta \in R(f)}\: q^\top \delta  \\
    & = \min_\delta \: ((\ones - 2f) \circ q )^\top \delta ~:~ \delta \in \{0,1\}^m , \;\; \ones^\top \delta \le p \\
    &=-s_p (((2f-\ones)\circ q )_+),
\end{align}
with $s_p$ the sum of the $p$ largest entries in its vector argument. To see why this is true, note that $\delta \in \{(\ones- 2f) \cup \textbf{0} \; | \; \|\delta\|_1 \leq p\}$. Hence we can either set $\delta_i =0$ or $\delta_i = (\ones - 2f)_i$; the optimal choice will clearly depend on the sign of $q_i$ and the result follows.
% The above problem can be solved by first sorting from largest to smallest (in absolute value) the entries of $\log \tp/(1-\tp)$ and proceeding as follows: check the entry of $f$ at the corresponding index and see if we can set $\delta_i = -\text{sign}(f_i)$ else move onto the next entry. We do this until we reach the end of until we have done this $s$ times in total to satisfy the $\|\delta\|_1 \le\tp s$ constraint.\\

Returning to the original max-min problem, we have that \eqref{eq:r-bnb-flip} becomes
\begin{align*}
    \max_{\tp,\tm \in [0,1]^m} &\;\;\;\;\fpt \log \tp + (\ones - \fp)^\top \log (\ones - \tp)  - s_p (((2\fp - \ones)\circ \log (\tp/ (1-\tp)) )_+) \\
    &+\fmt \log \tm + (\ones - \fm)^\top \log (\ones - \tm) - s_p (((2\fm - \ones)\circ \log (\tm/ (1-\tm)) )_+).
\end{align*}
This problem is convex, since the inner minimization is the pointwise minimum of jointly concave functions in $(\tp,\tm)$.

\paragraph{Multinomial model with typo uncertainty.}
Under the typo uncertainty, \eqref{eq:r-mnb} becomes
\begin{align*}
    \max_{\tp,\tm \in [0,1]^m} \: \min_{\delta_\pm \in R(\fpm)} &(\fp + \delta_+)^\top \log \tp + (\fm + \delta_-)^\top \log \tm ~:~ \ones^\top \tp = 1, \;\; \ones^\top \tm = 1 ,
\end{align*}
where 
\[
R(f_i) = \left\{ \delta ~:~ \delta + f_i \in \mathbb{N}^m, \; \|\delta\|_1 \leq t \right\} .
\]

Since the uncertainty acts independently on $\fp$ and $\fm$ we can consider the sub-problem
\begin{align*}
    \min_{\delta \in r(f)} (f+\delta)^\top \log \tp = f^\top \log \tp +  \min_{\delta \in r(f)} \delta^\top \log \tp 
\end{align*}
Note since the objective function above is linear, we can perform the minimization over the convex hull of the feasible region. Since $f \geq 0$, it follows that $$\textbf{Co}(r(f)) = \{ \delta \:|\:\delta + f\geq 0, \|\delta\|_1 \leq t\}$$
In this reformulation, the solution to the minimization is trivial. Since $\tp \in [0,1]^m$, we have that $\log \tp \leq 0$ and to minimize the inner product $\delta^\top \log \tp$ we set $\delta = t \cdot e_j$ where $e_j$ is the $j$th unit basis vector and $j$ is the index corresponding to the largest absolute value entry of $\tp$. In summary, we have that
\begin{align*}
    \min_{\delta \in r(f)} \: \delta^\top \log \tp  = \min_{\delta \in \textbf{Co}(r(f))} \delta^\top \log \tp = -t \|\log \tp\|_\infty
\end{align*}
Returning to the original max-min problem, we have that \eqref{eq:r-mnb} becomes
\begin{align*}
    \max_{\tp,\tm \in [0,1]^m} & \fpt \log \tp + \fmt \log \tm  - t \Big( \| \log \tp \|_\infty + \| \log \tm\|_\infty \Big)\\
    & \text{s.t} \;\; \ones^\top \tp = 1, \;\; \ones^\top \tm = 1
\end{align*}
Note by monotonicity of the logarithm and positivity of $\tp,\tm$, the problem is equivalent to 
\begin{align*}
    \max_{\tp,\tm \in [0,1]^m} & \fpt \log \tp + \fmt \log \tm  - t \Big(  |\log (\dsp\max_{1 \le i \le m} \: \tp_i)| + |\log (\dsp\max_{1 \le i \le m} \: \tm_i)| \Big)\\
    & \text{s.t} \;\; \ones^\top \tp = 1, \;\; \ones^\top \tm = 1
\end{align*}
By construction, the problem is convex.

Note that the above problem is separable across $\tp,\tm$. We now show how to reduce the problem with typo uncertainty into a one dimensional problem that can be solved using bisection. Let
\begin{align*}
    p^\ast = \max_{\theta \in \Delta^m} \; f^\top \log \theta - t |\log (\dsp\max_{1 \le i \le m} \: \theta_i)|
\end{align*}
where $\Delta^m$ denote the simplex in $\mathbb{R}^m$. Then we have that
\begin{align*}
    p^\ast &= \max_{\substack{\theta \in \Delta^m\\  \log \theta \geq z\ones}} \; f^\top \log \theta + tz \\
    &= \min_\nu \max_{\substack{\theta \geq 0\\ \log \theta \geq z \ones}} \; f^\top \log \theta + tz + \nu (1 - \ones ^\top \theta) \\
    &= \min_\nu \max_{\substack{\theta \geq 0\\ \theta \geq u\ones}} \; f^\top \log \theta + t\log u + \nu (1 - \ones ^\top \theta)
\end{align*}
where the second equality follows by forming the lagrangian and using strong duality, the third line we make the substitution $u = e^z$. We first solve the inner maximization over $\theta$. The subproblem writes
\begin{align*}
    \max_{\theta \geq u\ones} \; f^\top \log \theta - \nu \ones^\top \theta
\end{align*}
Note if $\nu < 0$, then the problem is unbounded; hence $\nu \geq 0$. We then have that
\begin{align*}
    \theta^\ast = \max\Big( \dfrac{f}{\nu}, u\ones \Big)
\end{align*}
As a result, we have that $\max_i f_i := F \leq \nu$ amd $u \leq 1$ to ensure that $\theta^\ast_i \leq 1$ for all $i \in [m]$. Plugging back into the objective and rearranging we have
\begin{align*}
    p^\ast &= \min_{F \leq \nu} \max_{u \in [0,1]} \; f^\top \log \Big(\max(f/\nu,u\ones)\Big) + t\log u + \nu(1 - \ones^\top \max(f/\nu,u\ones)) \\
    &= \min_{F \leq \nu} \max_{u \in [0,1]} \; f^\top \log \Big(\max(f,\nu u\ones)\Big) - f^\top \ones \log \nu + t\log u + \nu - \ones^\top \max(f, \nu u\ones) \\
    &= \min_{F \leq \nu} \max_{\eta \in [0,\nu]} \; f^\top \log \Big(\max(f,\eta\ones)\Big) - f^\top \ones \log \nu + t\log \eta/\nu  + \nu - \ones^\top \max(f, \eta \ones) \\
    % &= \min_{\nu \in [F,\ones^\top f]} \max_{u \in [1/m,1]} \; f^\top \min(\log f - \log\nu \ones,\log u\ones) + t\log u + \nu - \ones^\top \min(f,\nu u\ones) \\
    % &= \min_{\nu \in [F,\ones^\top f]} \max_{u \in [1/m,1]} \; f^\top \min(\log f,\log \nu u \ones) - f^\top \ones \log \nu + t\log u + \nu - \ones^\top \min(f,\nu u\ones) \\
    % &= \min_{\nu \in [F,\ones^\top f]} \max_{\eta \in [\nu/m,\nu]} \; f^\top \min(\log f,\log \eta \ones) - f^\top \ones \log \nu + t\log \eta/\nu + \nu - \ones^\top \min(f,\eta\ones) \\
    % &= \max_{\eta \in H} \; f^\top \min(\log f,\log \eta \ones)- \ones^\top  \min(f,\eta\ones)  + t\log \eta + \min_{\nu \geq F} - f^\top \log \nu \ones + \nu - t \log \nu\\
    % &= \max_{\eta \in H} \; f^\top \min(\log f,\log \eta \ones)- \ones^\top  \min(f,\eta\ones)  + t\log \eta + C\\
\end{align*}

% We then arrive at
% \begin{align*}
%     p^\ast = \min_{\nu \in [F,\ones^\top f]} f^\top \min (\log f, \log \nu \ones) - f^\top \ones \log \nu + \nu - \ones^\top \min(f,\nu \ones)
% \end{align*}

\paragraph{Multinomial model with shift uncertainty.}
Under the shift uncertainty, \eqref{eq:r-mnb} becomes
\begin{align*}
    \max_{\tp,\tm \in [0,1]^m} \min_{\delta_i \in r(f_i)} &(\fp + \delta_+)^\top \log \tp + (\fm + \delta_-)^\top \log \tm \\
    & \text{s.t} \;\; \ones^\top \tp = 1, \;\; \ones^\top \tm = 1
\end{align*}
where $$r(f_i) = \{ \delta \; | \; \delta + f_i \in \mathbb{N}^m, \; \delta \in [-\gamma,\gamma]^m \cap \mathbb{Z}^m\}$$

Since the uncertainty acts independently on $\fp$ and $\fm$ we can consider the sub-problem
\begin{align*}
    \min_{\delta \in r(f)} (f+\delta)^\top \log \tp = f^\top \log \tp +  \min_{\delta \in R(f)} \delta^\top \log \tp 
\end{align*}
Since the objective function above is linear, we can perform the minimization over the convex hull of the feasible set. Since $f \geq 0$, it follows that $$\textbf{Co}(r(f)) = \{ \delta \:|\: \delta + f \geq 0, \; \|\delta\|_\infty \leq \gamma\}$$
In this reformulation, the solution to the minimization is trivial. Since $\tp \in [0,1]^m$, we have that $\log \tp \leq 0$ and in order to minimize the inner product, we simply set $\delta = \gamma \ones$ (note $\gamma \ones + f \geq 0$ since $f \geq 0$). In summary, we have that
\begin{align*}
   \min_{\delta \in r(f)} \delta^\top \log \tp  = \min_{\delta \in \textbf{Co}(r(f))} \delta^\top \log \tp = -\gamma \|\log \tp\|_1 = \gamma \sum_{i=1}^m \log \tp_i 
\end{align*}

returning to the original max-min problem, we have that \eqref{eq:r-mnb} becomes
\begin{align*}
    \max_{\tp,\tm \in [0,1]^m} & (\fp + |C_1| \gamma \ones)^\top \log \tp + (\fm + |C_2| \gamma \ones)^\top \log \tm \\
    & \text{s.t} \;\; \ones^\top \tp = 1, \;\; \ones^\top \tm = 1
\end{align*}
which is a convex problem (recall $|C_1|$ and $|C_2|$ are the number of data points in class 1 and class 2 in the training set).

Note the parallel between $\mathcal{V}_\text{shift}(x)$ and traditional Laplace smoothing for the Multinomial Naive Bayes model. If we assume $|C_1| = |C_2|$ and scale $\gamma$ by $1/|C_1|$, then the solution to the above problem is simply the MLE estimate and is
\begin{align*}
    \tpm^\ast = \dfrac{\fpm + \gamma \ones}{\sum_{i=1}^n (\fpm_i + \gamma)}
\end{align*}
which is the same performing Laplace smoothing with parameter $\gamma$. Similarly if $|C_1| \not = |C_2|$ we can set two different hyper parameters $\gamma_1, \gamma_2$ for each class and scale them by $1/|C_1|$ and $1/|C_2|$ to get the same formula as for traditional Laplacian smoothing for Multinomial Naive Bayes.
