# Supplementary material for: Naive Feature Selection: a Nearly Tight Convex Relaxation for Sparse Naive Bayes
Source: arXiv:1905.09884 source file (2025-03-12)
Supplement: Supplementary file 5 [file appendixE.tex]

% Writing the epigraph of problem~\eqref{eq:ncvx-pb-const},
% \[
% \mathcal{G}\triangleq \left\{(x,r_0,r) \in \reals^{d+1+m} :~ \sum_{i=1}^{n} f_i(x_i) \leq r_0,\,\sum_{i = 1}^n g_i(x_i) \leq r \right\},
% \]
% and its projection on the last $m+1$ coordinates,
% \BEQ\label{eq:epi}
% \mathcal{G}_r\triangleq \left\{(r_0,r) \in \reals^{m+1} :~  (x,r_0,r)\in \mathcal{G}\right\},
% \EEQ
% we can write the Lagrange dual function of~\eqref{eq:ncvx-pb-const} as 
% \BEQ\label{eq:dual-f}
% \Psi(\lambda) \triangleq \inf\left\{ r_0 + \lambda^{\top}r:~ (r_0,r) \in \mathcal{G}_r^{**} \right\},
% \EEQ
% in the variable $\lambda\in\reals^m$, where $\mathcal{G}^{**}=\overline{\Co(\mathcal{G})}$ is the closed convex hull of the epigraph $\mathcal{G}$ (the projection being linear here, we have $(\mathcal{G}_r)^{**}=(\mathcal{G}^{**})_r=\mathcal{G}_r^{**}$). The dual takes the generic form
% \BEQ\label{eq:dual-pb-const}\tag{cD}
% \sup_{\lambda \geq 0} \Psi(\lambda),
% \EEQ
% where $\Psi$ is the dual function associated to problem~\eqref{eq:ncvx-pb-const}. Note that explicitly deriving this dual may be hard. %We let $\mathrm{h}_{cD} \triangleq \mathrm{h}_{cP}^{**}$ be the dual of problem~\eqref{eq:p-ncvx-pb-const} and in particular, solving for $\mathrm{h}_{cD}(0)$ is equivalent to solving problem~\eqref{eq:dual-pb-const}. 


% Using these new definitions, we can formulate a more general bound for the duality gap (see \cite[Appendix I, Thm. 3]{Ekel99} for more details).
% \begin{proposition}
% Suppose the functions $f_i$ and $g_i$ in~\eqref{eq:ncvx-pb-const} are such that all $(f_i + \ones^{\top} g_i)$ satisfy Assumption~\ref{as:fi}. Then, one has
% \[
%   \mathrm{h}_{cD}((m + 1)\bar{\rho}_g) \leq \mathrm{h}_{cP}((m + 1) \bar{\rho}_g) \leq \mathrm{h}_{cD}(0) + (m + 1) \bar{\rho}_f,
% \]
% where $\bar{\rho}_f = \sup_{i \in [1,n]} \rho(f_i)$ and $\bar{\rho}_g = \sup_{i \in [1, n]} \rho(g_i)$.
% \end{proposition}
% \begin{proof}
% Let us write
% \[
% \mathcal{F}_i = \left\{ \left(f_i(x_i), g_i(x_i) \right):~ x_i \in \reals^{d_i} \right\},
% \]
% we have, because the sets $\Co(\mathcal{F}_i)$ closed by Assumption~\ref{as:fi},
% \[
% \mathcal{G}_r^{**} = \sum_{i=1}^n \Co(\mathcal{F}_i).
% \]
% Now, the Shapley-Folkman theorem \citep{Star69} shows that we have in fact
% \[
% \mathcal{G}_r^{**} = \sum_{i\in [1,n] \setminus \mathcal{S}} \mathcal{F}_i + \sum_{i\in \mathcal{S}} \Co(\mathcal{F}_i)
% \]
% with $|\mathcal{S}|\leq m+1$. With $\mathcal{G}_r^{**}$ closed by construction, this means that there are points $x_i\in\reals^{d_i}$, for $i\in [1,n] \setminus \mathcal{S}$ and $x_{ij}\in\reals^{d_i}$, for $i\in [1,n] \setminus \mathcal{S}$, $j\in 1,\ldots,m+1$ together with coefficients $\mu_{ij}\geq 0$ such that $\ones^T\mu_i=1$, and the corresponding minimizer of~\eqref{eq:dual-f} in $\mathcal{G}_r^{**}$  can be written
% \BEQ\label{eq:zstar}
% z^\star = \sum_{i\in [1,n] \setminus \mathcal{S}}
% \begin{pmatrix}
% f_i(x_i)\\
% g_i(x_i)
% \end{pmatrix}
% +
% \sum_{i\in \mathcal{S}}
% \sum_{j\in [1,m+1]}
% \mu_{ij} \begin{pmatrix}
% f_i(x_{ij})\\
% g_i(x_{ij})
% \end{pmatrix}
% +
% \begin{pmatrix}
% 0\\
% w
% \end{pmatrix}
% \EEQ
% with $w \in \reals^{m}_+$. Since $z^\star_1=\Psi(\lambda^\star)$, calling $x_i=\sum_{j=1}^{m+1}\mu_{ij}x_{ij}$, this means in particular
% \BEAS
% \Psi(\lambda^\star) &=& \sum_{i\in [1,n] \setminus \mathcal{S}} f_i(x_i) + \sum_{i\in \mathcal{S}}f_i(x_i) + \sum_{i\in\mathcal{S}}\left(\sum_{j=1}^{m+1}\mu_{ij} f_i(x_{ij}) - f_i(x_i) \right)\\
% & \geq &  \sum_{i\in [1,n] \setminus \mathcal{S}} f_i(x_i) + \sum_{i\in \mathcal{S}}f_i(x_i) - \sum_{i\in \mathcal{S}} \rho(f_i)\\
% & \geq &  \sum_{i=1}^n f_i(x_i) - \sum_{i\in \mathcal{S}} \rho(f_i).
% \EEAS
% using~\eqref{def:alt-lack-cvx}. 

% \end{proof}
